# Supplementary material for: Proton and neutron density distributions at supranormal density in low- and medium-energy heavy-ion collisions
Source: arXiv:1706.01582 source file (2017-06-06)
Supplement: Supplementary file 1 [file Supplemental_material.pdf]

## I. SUMMARY OF COEFFICIENTS OF THE INTERPOLATION FUNCTION

We have interpolated the maximum proton and neutron densities as a function of beam energy as calculated in the S, SM, SMS, SSM, Vlasov (V) and TDHF models using a function $y = a_0 + a_1 \log(1 + a_2 x)$, with $y$ being the density and $x$ the beam energy per nucleon in the laboratory system in MeV/nucl. The parameters are reasonably consistent for each model showing that the adopted interpolation function is adequate for description of the data.

TABLE I: Coefficients $a_0$, $a_1$ and $a_2$ of the empirical function used to interpolate the maximum proton and neutron density as a function of beam energy for all systems studied in this work in the pBUU, Vlasov and TDHF models. The error is relative r.m.s deviation in percent.

| System | $\rho_{\rm n}^{\rm max}$ | | | | $\rho_{\rm p}^{\rm max}$ | | | |
|---|---|---|---|---|---|---|---|---|
| | $a_0$ | $a_1$ | $a_2$ | error | $a_0$ | $a_1$ | $a_2$ | error |
| | $fm^{-3}$ | $fm^{-3}$ | $MeV^{-1}$ | % | $fm^{-3}$ | $fm^{-3}$ | $MeV^{-1}$ | % |
| S | | | | | | | | |
| 4848 | 0.5186 | 0.1270 | 0.2141 | 2.49 | 0.4155 | 0.0984 | 0.3129 | 3.25 |
| 4048 | 0.5183 | 0.1128 | 0.2241 | 2.68 | 0.4566 | 0.0963 | 0.2894 | 2.01 |
| 4040 | 0.4801 | 0.1167 | 0.2111 | 2.74 | 0.4622 | 0.1205 | 0.1683 | 2.42 |
| 100100 | 0.4787 | 0.1327 | 0.1985 | 3.21 | 0.4474 | 0.1293 | 0.1549 | 3.58 |
| 100120 | 0.5201 | 0.1552 | 0.1105 | 3.28 | 0.4403 | 0.1280 | 0.1201 | 3.42 |
| 120120 | 0.5189 | 0.1584 | 0.1264 | 3.62 | 0.3887 | 0.1216 | 0.1642 | 3.50 |
| SM | | | | | | | | |

Table Continued on Next Page...

TABLE I – Continued

| System | $\rho_n^{max}$ | | | | $\rho_p^{max}$ | | | |
|---|---|---|---|---|---|---|---|---|
| | $a_0$ | $a_1$ | $a_2$ | error | $a_0$ | $a_1$ | $a_2$ | error |
| | $fm^{-3}$ | $fm^{-3}$ | $MeV^{-1}$ | % | $fm^{-3}$ | $fm^{-3}$ | $MeV^{-1}$ | % |
| 4848 | 0.5269 | 0.1615 | 0.1311 | 2.43 | 0.4031 | 0.1259 | 0.1624 | 2.72 |
| 4048 | 0.5241 | 0.1336 | 0.1774 | 2.65 | 0.4580 | 0.1251 | 0.1443 | 2.18 |
| 4040 | 0.4781 | 0.1357 | 0.1638 | 2.82 | 0.4596 | 0.1281 | 0.1694 | 2.20 |
| 100100 | 0.4717 | 0.1608 | 0.1194 | 1.88 | 0.4440 | 0.1498 | 0.0971 | 2.30 |
| 100120 | 0.5376 | 0.1676 | 0.0992 | 1.99 | 0.4371 | 0.1464 | 0.0803 | 3.07 |
| 120120 | 0.5271 | 0.1768 | 0.1168 | 1.95 | 0.3855 | 0.1240 | 0.1400 | 1.45 |
| SMS | | | | | | | | |
| 4848 | 0.5219 | 0.1484 | 0.1402 | 1.72 | 0.4049 | 0.1283 | 0.1610 | 1.94 |
| 4048 | 0.5195 | 0.1296 | 0.1608 | 1.62 | 0.4560 | 0.1144 | 0.2028 | 1.58 |
| 4040 | 0.4753 | 0.1279 | 0.1929 | 2.43 | 0.4596 | 0.1222 | 0.1965 | 1.75 |
| 100100 | 0.4699 | 0.1519 | 0.1370 | 1.67 | 0.4396 | 0.1420 | 0.1210 | 1.81 |
| 100120 | 0.5212 | 0.1657 | 0.0962 | 1.92 | 0.4402 | 0.1362 | 0.1064 | 1.67 |
| 120120 | 0.5266 | 0.1761 | 0.0987 | 2.70 | 0.3818 | 0.1398 | 0.1149 | 1.56 |
| SSM | | | | | | | | |
| 4848 | 0.5164 | 0.1165 | 0.1050 | 1.19 | 0.4146 | 0.1175 | 0.1747 | 1.63 |
| 4048 | 0.5171 | 0.1294 | 0.1989 | 1.60 | 0.4560 | 0.1105 | 0.2256 | 1.06 |
| 4040 | 0.4761 | 0.1305 | 0.1922 | 2.24 | 0.4586 | 0.1234 | 0.2060 | 1.47 |
| 100100 | 0.4719 | 0.1567 | 0.1325 | 1.95 | 0.4403 | 0.1393 | 0.1189 | 2.03 |

Table Continued on Next Page...

TABLE I – Continued

| System | $\rho_{\rm n}^{\rm max}$ | | | | $\rho_{\rm p}^{\rm max}$ | | | |
|---|---|---|---|---|---|---|---|---|
| | $a_0$ | $a_1$ | $a_2$ | error | $a_0$ | $a_1$ | $a_2$ | error |
| | fm$^{-3}$ | fm$^{-3}$ | MeV$^{-1}$ | % | fm$^{-3}$ | fm$^{-3}$ | MeV$^{-1}$ | % |
| 100120 | 0.5178 | 0.1662 | 0.1066 | 1.71 | 0.4466 | 0.1499 | 0.0735 | 2.37 |
| 120120 | 0.5242 | 0.1761 | 0.1159 | 2.49 | 0.3945 | 0.1382 | 0.1002 | 2.15 |
| V | | | | | | | | |
| 4848 | 0.5139 | 0.0929 | 0.5690 | 1.98 | 0.4140 | 0.0789 | 0.6554 | 3.08 |
| 4048 | 0.5119 | 0.0869 | 0.5962 | 2.14 | 0.4562 | 0.0771 | 0.6545 | 3.03 |
| 4040 | 0.4767 | 0.0927 | 0.4960 | 3.00 | 0.4571 | 0.0868 | 0.5404 | 3.34 |
| 100100 | 0.4679 | 0.0894 | 0.5816 | 3.61 | 0.4346 | 0.0829 | 0.5228 | 3.37 |
| 100120 | 0.5069 | 0.0874 | 0.6115 | 2.31 | 0.4331 | 0.0767 | 0.5537 | 4.39 |
| 120120 | 0.5105 | 0.0932 | 0.6186 | 2.85 | 0.3835 | 0.0735 | 0.8116 | 3.38 |
| TDHF | | | | | | | | |
| 4040 | 0.5500 | 0.2532 | 0.0215 | 0.86 | 0.5272 | 0.2787 | 0.0149 | 0.82 |
| 4048 | 0.5527 | 0.1430 | 0.0703 | 0.89 | 0.5117 | 0.2007 | 0.0191 | 0.89 |
| 4848 | 0.5585 | 0.0916 | 0.1972 | 0.30 | 0.47951 | 0.4028 | 0.0086 | 0.64 |
| 100100 | 0.4730 | 0.1527 | 0.0798 | 1.28 | 0.4433 | 0.0733 | 0.3035 | 0.60 |
| 100120 | 0.5534 | 0.1216 | 0.0977 | 1.52 | 0.4221 | 0.0471 | 0.7099 | 0.61 |
| 120120 | 0.5980 | 0.4148 | 0.0167 | 1.75 | 0.4003 | 0.0542 | 0.2333 | 1.22 |
